# Supplementary material for: $\nu$-LPA: Fast GPU-based Label Propagation Algorithm (LPA) for Community Detection
Source: arXiv:2411.11468 source file (2025-01-06)
Supplement: Supplementary file 1 [file aa-appendix.tex]

\section{Appendix}

\subsection{Indirect Comparison with State-of-the-art Leiden Implementations}
\label{sec:comparison-indirect}

% Finally, we conduct an indirect comparison of the performance of our multicore implementation of the Leiden algorithm with other similar state-of-the-art implementations, as listed in Table \ref{tab:compare}. Please consider the reported speedups as approximate. Hu et al. \cite{huparleiden} introduce ParLeiden, a parallel Leiden implementation for distributed environments, which uses thread locks and efficient buffers, to resolve community joining conflicts and reduce communication overheads. They refer to their single node version of ParLeiden as ParLeiden-S, and their distributed version as ParLeiden-D. On a cluster with $8$ nodes, with each node being equipped with a $48$ core CPU, Hu et al. observe a speedup of $12.3\times$, $9.9\times$, and $1.32\times$ for ParLeiden-S, ParLeiden-D, and a baseline Leiden implemented on KatanaGraph, on the \textit{com-LiveJournal} graph, with respect to original Leiden \cite{com-traag19} (refer to Table 2 in their paper \cite{huparleiden}). In contrast, on the same graph, we observe a speedup of $219\times$ relative to original Leiden. Consequently, GVE-Leiden outperforms ParLeiden-S, ParLeiden-D, and KatanaGraph Leiden by approximately $18\times$, $22\times$, and $166\times$ respectively\ignore{ (all achieved without GPU)}.

\begin{figure}[hbtp]
  \centering
  \subfigure{
    \label{fig:optcoalesced--runtime}
    \includegraphics[width=0.98\linewidth]{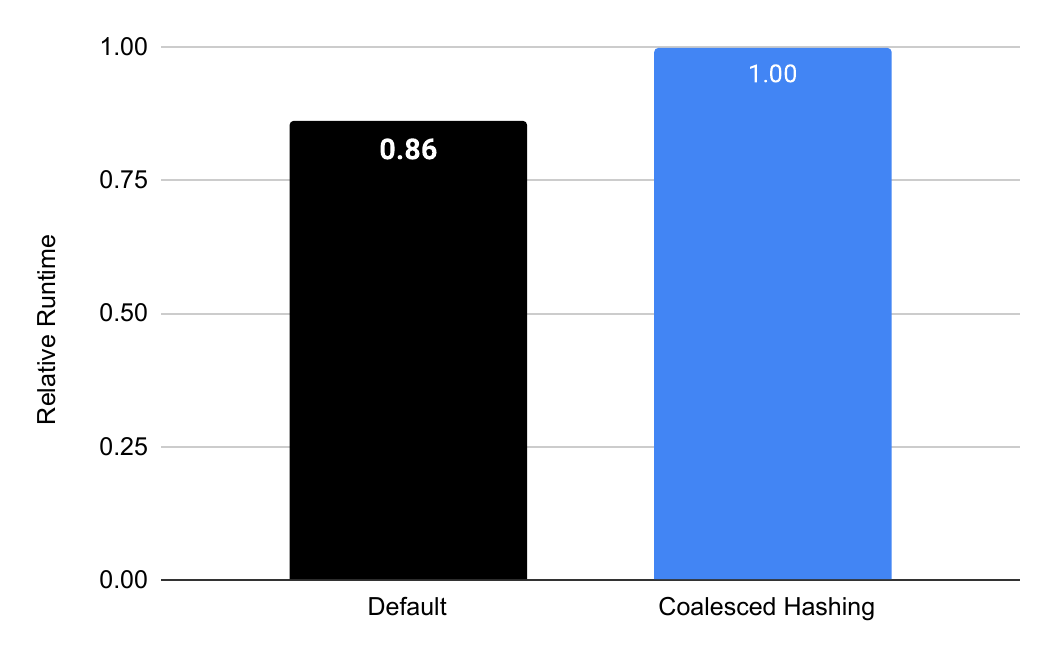}
  } \\[-2ex]
  \caption{Relative Runtime for our current approach for hashtable (\textit{Default}), compared to a hashtable based on 
\textit{Coalesced Hashing}.}
  \label{fig:optcoalesced}
\end{figure}

%% A description of how the cross-check approach works, but no algorithm.
